# Supplementary material for: Landmarks and Regions: A Robust Approach to Data Extraction
Source: arXiv:2204.05021 source file (2022-04-11)
Supplement: Supplementary file 1 [file appendix.tex]

\section{Region program for HTML}
\begin{algorithm}
\small
\caption{$\mathsf{LearnRegionProgram}$ for a HTML document}
\label{algo:regionhtml}
\begin{algorithmic}[1]
\Require Annotated HTML documents $D_{tr}$ from a single cluster 
\Require Field values $f_T(d)$ \spsays{Do we remove the field here as well?}
\Require $\ell^{f_T}_d$
\State $\mathsf{BluePrint} \gets \langle\rangle$
\State $\mathsf{Hops} \gets \langle\rangle$
\For {$Document \; d \in D_{tr}$}
\State $\mathsf{ParentHops}, \mathsf{SiblingHops} \gets 0, 0$
\State $\mathsf{landmarkRegion} \gets \locate({\ell^{f_T}_d})$
\State $\mathsf{fieldRegions} \gets f_T(d)$
\State $\mathsf{region} \gets \mathsf{landmarkRegion}$
\Do
    \If{$\forall \; \mathsf{fieldRegions} \subseteq \mathsf{region}$}
    \State break
    \EndIf
    \If{$\forall \; \mathsf{fieldRegions}$ are k siblings from $\mathsf{region}$}
    \State $\mathsf{SiblingHops} \gets k$
    \State break
    \EndIf
    \State $\mathsf{ParentHops} \gets \mathsf{ParentHops} + 1$
    \State $\mathsf{region} \gets \mathsf{Expand} \; \mathsf{region}$ by one parent
\doWhile {$\mathsf{True}$}
\State $\mathsf{Hops} \gets \mathsf{Hops} + \langle \mathsf{ParentHops}, \mathsf{SiblingHops} \rangle$
\EndFor
\State
\State ParentHops = max over all parenthops in Hops \spsays{Write this formally}
\State SiblingHops = max over all siblinghops for parenthop == ParentHops found above
\State
\State $\mathsf{BluePrint} \gets \bprint(P_{rg}(d))$ \spsays{we take blueprints over all documents and maintain them as set, usually the size is <=3. Should we simplify this?}
\State
\State $P_{rg} \gets \mathsf{ParentHops}, \mathsf{SiblingHops} , \mathsf{BluePrint}$
\State \Return $P_{rg}$
\end{algorithmic}
\end{algorithm}

Algorithm~\ref{algo:regionhtml}~describes the region growing algorithm for a HTML document. The algorithm loops through the training documents $D_{tr}$ and for each document, finds the $\mathsf{ParentHops}$ and $\mathsf{SiblingHops}$ required to grow the region. The first step in the algorithm (Line 5) is to use the $\locate$ function to find the region associated with the landmark value. In this case, $\locate$ function translates to a simple \emph{grep} on the document. We initialize the $region$ variable to encompass the landmark region (Line 7).

The algorithm proceeds as follows: We check if all the field regions are contained within the $region$ itself, in which case we are done. Else, we check if all the field regions are within $k$ siblings away from the region. We call this as the \emph{sibling consistency} check. If this check passes, we set $\mathsf{SiblingHops}$ to $k$ and break. Else, it implies that we need a larger region to encompass the landmark and field regions. We increment the $\mathsf{SiblingHops}$ by $1$ and expand the region by one parent (Lines $14 \to 15$) and continue with the iteration from Line $9$.

At the end of the loop, we have $\mathsf{ParentHops}$ and $\mathsf{SiblingHops}$ across all training documents $D_{tr}$. Since we require a common parameter which will work across documents during inference time, we reconcile these two parameters as follows: We take the maximum over $\mathsf{ParentHops}$. Lets call this $M$. And for all pairs with $\mathsf{ParentHops} == M$, we take the maximum over $\mathsf{SiblingHops}$. Theorem~\ref{}~proves that this operation always computes the required region correctly across all documents.

In addition to the hops, we also output a blueprint characterizing the region. For doing this, we again grow the regions for each document using the final $\mathsf{ParentHops}$ and $\mathsf{SiblingHops}$ and add the resulting region blueprints to a set and return them.

\begin{theorem}
The operation described above to reconcile $\mathsf{ParentHops}$ and $\mathsf{SiblingHops}$ always produces the correct region for the given input documents.

\spsays{Write this formally}

Example: If we have (3, 0) and (2, 1), this will result in (3, 0). And (3, 0) will be a superset of the region and will contain (2, 1) as well.

Likewise, if we have (3, 0) and (3, 1), if we take the region (3, 1), it will also contain (3, 0). 

\end{theorem}

{\bf[MOHAMMAD COMMENT: ] It is not clear what "correct" here means. Do you mean a region that contains the desired field values and landmark values? If so, then that sounds more like a soundness result that many possible answers could satisfy rather than one "correct" answer. So may be good to reword the theorem to "a correct region". Also wonder if theorem could be made stronger - e.g. is it the "smallest" such region or something like that? }

\begin{figure}
\small
\begin{tabular}{r c l}
Prog & := & \textsf{map}(\(\lambda\) node .\; \textsf{FFProg}(node), \textsf{Nodes}) \\
Nodes & := & \textsf{AllNodes}(\textsf{input}) | \textsf{Descendants}(\textsf{Nodes}) \\
     &  &    | \textsf{filter}(\textsf{Selector}, \textsf{Nodes}) | \textsf{Children}(\textsf{Nodes}) \\
Selector & := & \textbf{tag} = c | \textbf{class} = c | \textbf{id} = c | \textbf{nth-child}(n) | \ldots \\
FFProg & := & \textsf{Substring} | \textsf{Concat}(\textsf{SubString}, \textsf{FFProg}) \\
SubString & := & \textsf{node.TextValue}  \\
          &    & | \textsf{Extract}(RegexPos, RegexPos, SubString) \\
RegexPos & := & \textsf{RegexSearch}(\textit{regex}, k)
\end{tabular}
\vspace{-2ex}
\caption{Syntax of the HTML extraction language $\LL_{ex}$}
\vspace{-3ex}
\end{figure}

\begin{table*}[ht]
\small
\label{table:m2hexpmt1}
\resizebox{8cm}{!}{
\begin{tabular}{|c|l|c|c|c|c|c|c|c|c|}
\hline
{Domain} & Fields & \multicolumn{4}{|c|}{$\ndsyn$} & \multicolumn{4}{|c|}{$\resyn$}\\
\cline{3-10}&  & Prgs & Pre. & Rec. & F1 & Prgs & Pre. & Rec. & F1\\
\hline
\hline\multirow{8}{*}{ifly.alaskaair.com}

& AIata & 2 & 0.99 & 0.47 & 0.64 & 1 & 1.00 & 1.00 & 1.00 \\
& ATime & 2 & 0.97 & 0.46 & 0.62 & 1 & 1.00 & 1.00 & 1.00 \\
& DIata & 2 & 0.89 & 0.42 & 0.57 & 1 & 1.00 & 1.00 & 1.00 \\
& DDate & 1 & 1.00 & 1.00 & 1.00 & 2 & 1.00 & 1.00 & 1.00 \\
& DTime & 2 & 0.89 & 0.42 & 0.58 & 1 & 1.00 & 1.00 & 1.00 \\
& FNum  & 1 & 1.00 & 1.00 & 1.00 & 1 & 1.00 & 1.00 & 1.00 \\
& Name  & 1 & 1.00 & 0.99 & 0.99 & 1 & 1.00 & 0.99 & 0.99 \\
& RId   & 1 & 1.00 & 1.00 & 1.00 & 1 & 1.00 & 1.00 & 1.00 \\

\hline\multirow{9}{*}{delta.com}

& AIata & 2 & 1.00 & 1.00 & 1.00 & 2 & 1.00 & 1.00 & 1.00 \\
& ATime & 2 & 1.00 & 1.00 & 1.00 & 2 & 1.00 & 1.00 & 1.00 \\
& DIata & 2 & 1.00 & 1.00 & 1.00 & 2 & 1.00 & 1.00 & 1.00 \\
& DDate & 1 & 0.94 & 0.97 & 0.95 & 2 & 1.00 & 1.00 & 1.00 \\
& DTime & 2 & 1.00 & 1.00 & 1.00 & 2 & 1.00 & 1.00 & 1.00 \\
& FNo   & 2 & 1.00 & 1.00 & 1.00 & 2 & 1.00 & 1.00 & 1.00 \\
& Name  & 2 & 0.95 & 0.88 & 0.91 & 2 & 0.95 & 1.00 & 0.97 \\
& Pvdr  & 2 & 1.00 & 1.00 & 1.00 & 2 & 1.00 & 1.00 & 1.00 \\
& RId   & 2 & 1.00 & 0.99 & 0.99 & 2 & 1.00 & 0.99 & 0.99 \\

\hline\multirow{9}{*}{booking.airasia.com}

& AIata & 1 & 0.67 & 1.00 & 0.67 & 1 & 1.00 & 1.00 & 1.00 \\
& ATime & 0 & 0.00 & 0.00 & 0.00 & 1 & 1.00 & 1.00 & 1.00 \\
& DIata & 1 & 0.67 & 1.00 & 0.67 & 1 & 1.00 & 1.00 & 1.00 \\
& DDate & 1 & 0.67 & 1.00 & 0.67 & 1 & 1.00 & 1.00 & 1.00 \\
& DTime & 0 & 0.00 & 0.00 & 0.00 & 1 & 1.00 & 1.00 & 1.00\\
& FNo   & 1 & 1.00 & 0.92 & 0.92 & 1 & 1.00 & 0.92 & 0.92 \\
& Name  & 1 & 1.00 & 1.00 & 1.00 & 1 & 1.00 & 1.00 & 1.00 \\
& Pvdr  & 1 & 1.00 & 0.92 & 0.92 & 1 & 1.00 & 0.92 & 0.92 \\
& RId   & 1 & 1.00 & 1.00 & 1.00 & 1 & 1.00 & 1.00 & 1.00 \\

\hline\multirow{9}{*}{getthere.com}

& AIata & 3 & 0.73 & 0.84 & 0.78 & 1 & 1.00 & 1.00 & 1.00 \\
& ATime & 2 & 0.94 & 0.91 & 0.92 & 1 & 1.00 & 1.00 & 1.00 \\
& DIata & 3 & 0.94 & 0.95 & 0.94 & 1 & 1.00 & 1.00 & 1.00 \\
& DDate & 3 & 0.98 & 0.94 & 0.96 & 1 & 1.00 & 1.00 & 1.00 \\
& DTime & 2 & 0.86 & 0.85 & 0.85 & 1 & 1.00 & 1.00 & 1.00 \\
& FNo   & 1 & 0.94 & 0.96 & 0.95 & 1 & 1.00 & 1.00 & 1.00 \\
& Name  & 1 & 0.83 & 0.96 & 0.89 & 1 & 1.00 & 1.00 & 1.00 \\
& Pvdr  & 1 & 0.98 & 0.95 & 0.97 & 1 & 1.00 & 1.00 & 1.00 \\
& RId   & 1 & 1.00 & 0.88 & 0.94 & 1 & 1.00 & 1.00 & 1.00 \\

\hline\multirow{9}{*}{t.delta.com}

& AIata & 1 & 1.00 & 1.00 & 1.00 & 1 & 1.00 & 1.00 & 1.00 \\
& ATime & 1 & 0.99 & 1.00 & 0.99 & 1 & 0.99 & 1.00 & 0.99 \\
& DIata & 1 & 1.00 & 1.00 & 1.00 & 1 & 1.00 & 1.00 & 1.00 \\
& DDate & 1 & 1.00 & 1.00 & 1.00 & 1 & 1.00 & 1.00 & 1.00 \\
& DTime & 1 & 0.99 & 1.00 & 0.99 & 1 & 0.99 & 1.00 & 0.99 \\
& FNo   & 2 & 1.00 & 1.00 & 1.00 & 2 & 1.00 & 1.00 & 1.00 \\
& Name  & 1 & 0.99 & 0.99 & 0.99 & 1 & 0.99 & 0.99 & 0.99 \\
& Pvdr  & 2 & 0.99 & 0.97 & 0.98 & 2 & 1.00 & 0.97 & 0.98 \\
& RId   & 1 & 1.00 & 1.00 & 1.00 & 1 & 1.00 & 1.00 & 1.00 \\

\hline\multirow{9}{*}{philippineairlines.com}

& AIata  & 3 & 0.91 & 1.00 & 0.96 & 3 & 1.00 & 1.00 & 1.00 \\
& ATime  & 2 & 1.00 & 1.00 & 1.00 & 3 & 1.00 & 0.98 & 0.99 \\
& DIata  & 2 & 0.99 & 0.99 & 0.99 & 2 & 0.99 & 0.99 & 0.99 \\
& DeDate & 2 & 0.98 & 0.94 & 0.96 & 2 & 0.98 & 0.94 & 0.96 \\
& DTime  & 2 & 1.00 & 1.00 & 1.00 & 3 & 1.00 & 0.98 & 0.99 \\
& FNo    & 3 & 0.74 & 0.68 & 0.70 & 3 & 1.00 & 0.93 & 0.97 \\
& Name   & 3 & 1.00 & 0.97 & 0.99 & 2 & 1.00 & 0.99 & 0.99 \\
& Pvdr   & 2 & 1.00 & 1.00 & 1.00 & 2 & 1.00 & 1.00 & 1.00 \\
& RId    & 2 & 1.00 & 1.00 & 1.00 & 2 & 1.00 & 1.00 & 1.00 \\

\hline\multirow{9}{*}{itinerary.westjet.com}

& AIata & 1 & 1.00 & 1.00 & 1.00 & 1 & 1.00 & 1.00 & 1.00 \\
& ATime & 1 & 1.00 & 1.00 & 1.00 & 1 & 1.00 & 1.00 & 1.00 \\
& DIata & 1 & 1.00 & 1.00 & 1.00 & 1 & 1.00 & 1.00 & 1.00 \\
& DDate & 1 & 1.00 & 1.00 & 1.00 & 1 & 1.00 & 1.00 & 1.00 \\
& DTime & 1 & 1.00 & 1.00 & 1.00 & 1 & 1.00 & 1.00 & 1.00 \\
& FNo   & 1 & 1.00 & 1.00 & 1.00 & 1 & 1.00 & 1.00 & 1.00 \\
& Name  & 1 & 1.00 & 1.00 & 1.00 & 1 & 1.00 & 1.00 & 1.00 \\
& Pvdr  & 1 & 1.00 & 1.00 & 1.00 & 1 & 1.00 & 1.00 & 1.00 \\
& RId   & 1 & 1.00 & 1.00 & 1.00 & 1 & 1.00 & 1.00 & 1.00 \\

\hline\multirow{9}{*}{aeromexico.com}

& AIata & 1 & 1.00 & 1.00 & 1.00 & 1 & 1.00 & 1.00 & 1.00 \\
& ATime & 1 & 1.00 & 1.00 & 1.00 & 1 & 1.00 & 1.00 & 1.00 \\
& DIata & 1 & 1.00 & 1.00 & 1.00 & 1 & 1.00 & 1.00 & 1.00 \\
& DDate & 1 & 1.00 & 1.00 & 1.00 & 1 & 1.00 & 1.00 & 1.00 \\
& DTime & 1 & 1.00 & 1.00 & 1.00 & 1 & 1.00 & 1.00 & 1.00 \\
& FNo   & 1 & 1.00 & 1.00 & 1.00 & 1 & 1.00 & 1.00 & 1.00 \\
& Name  & 1 & 1.00 & 1.00 & 1.00 & 1 & 1.00 & 1.00 & 1.00 \\
& Pvdr  & 1 & 1.00 & 1.00 & 1.00 & 1 & 1.00 & 1.00 & 1.00 \\
& RId   & 1 & 1.00 & 1.00 & 1.00 & 1 & 1.00 & 1.00 & 1.00 \\

\hline\multirow{9}{*}{mytrips.amexgbt.com}
& AIata & 1 & 1.00 & 1.00 & 1.00 & 1 & 1.00 & 1.00 & 1.00 \\
& ATime & 1 & 0.99 & 0.99 & 0.99 & 1 & 1.00 & 1.00 & 1.00 \\
& DIata & 1 & 1.00 & 1.00 & 1.00 & 1 & 1.00 & 1.00 & 1.00 \\
& DDate & 1 & 0.99 & 1.00 & 0.99 & 1 & 1.00 & 1.00 & 1.00 \\
& DTime & 1 & 0.99 & 1.00 & 0.99 & 1 & 1.00 & 1.00 & 1.00 \\
& FNo   & 1 & 1.00 & 1.00 & 1.00 & 1 & 1.00 & 1.00 & 1.00 \\
& Name  & 1 & 1.00 & 1.00 & 1.00 & 1 & 1.00 & 1.00 & 1.00 \\
& Pvdr  & 1 & 1.00 & 1.00 & 1.00 & 1 & 1.00 & 1.00 & 1.00 \\
& RId   & 1 & 1.00 & 1.00 & 1.00 & 1 & 1.00 & 1.00 & 1.00 \\

\hline\multirow{9}{*}{qatarairways.com.qa}

& AIata & 1 & 1.00 & 1.00 & 1.00 & 1 & 1.00 & 1.00 & 1.00 \\
& ATime & 1 & 1.00 & 1.00 & 1.00 & 1 & 1.00 & 1.00 & 1.00 \\
& DIata & 1 & 1.00 & 1.00 & 1.00 & 1 & 1.00 & 1.00 & 1.00 \\
& DDate & 1 & 1.00 & 1.00 & 1.00 & 1 & 1.00 & 1.00 & 1.00 \\
& DTime & 1 & 1.00 & 1.00 & 1.00 & 1 & 1.00 & 1.00 & 1.00 \\
& FNo   & 1 & 0.99 & 1.00 & 0.99 & 1 & 0.99 & 1.00 & 0.99 \\
& Name  & 1 & 0.99 & 1.00 & 0.99 & 1 & 0.99 & 1.00 & 0.99 \\
& Pvdr  & 1 & 1.00 & 1.00 & 1.00 & 1 & 1.00 & 1.00 & 1.00 \\
& RId   & 2 & 1.00 & 0.99 & 0.99 & 2 & 1.00 & 1.00 & 1.00 \\

\hline
\end{tabular}
}
\caption{No. Program, Precision, Recall and F1 numbers on HTML extraction scenario (M2H dataset) with NDSyn and ReSyn}
\end{table*}

\begin{table*}[t]
\small
\label{table:m2hexpmt2appendix}
\begin{tabular}{|c|c|c|c|c|c|c|c|c|c|c|}
\hline
{Domain} & Fields & \multicolumn{4}{|c|}{HDEF} & \multicolumn{5}{|c|}{$\resyn$}\\
\cline{3-11}&  & Programs & Pre. & Rec. & F1 & Clusters & Programs & Pre. & Rec. & F1\\
\hline
\hline\multirow{9}{*}{delta.com}
& ArrivalAirportIata&2&0.9967&0.9967&0.9967&2&2&0.9967&0.9967&0.9967\\
& ArrivalTime&2&0.9962&0.9975&0.9968&2&3&0.9971&0.9975&0.9973\\
& DepartureAirportIata&2&0.9934&0.9967&0.9950&2&2&0.9934&0.9967&0.9950\\
& DepartureDate&2&0.932&0.9659&0.9486&2&2&0.9986&0.9977&0.9981\\
& DepartureTime&2&1&0.9975&0.9987&2&2&1&0.9975&0.9987\\
& FlightNumber&2&1&1&1.00&2&2&1&1&1.00\\
& Name&2&0.9447&0.8795&0.9109&3&3&0.951&1&0.9749\\
& Provider&2&1&1&1.00&2&2&1&1&1.00\\
& ReservationId&2&1&0.9989&0.9994&3&3&1&0.9989&0.9994\\
\hline\multirow{9}{*}{philippineairlines.com}
& ArrivalAirportIata&3&1&1&1.00&2&3&1&1&1.00\\
& ArrivalTime&2&1&1&1.00&2&3&1&1&1.00\\
& DepartureAirportIata&2&0.9937&0.9937&0.9937&2&2&0.9935&0.9935&0.9935\\
& DepartureDate&2&0.9815&0.9463&0.9636&2&2&0.9809&0.9449&0.9626\\
& DepartureTime&2&1&1&1.00&2&3&1&1&1.00\\
& FlightNumber&2&0.8983&1&0.9464&2&2&0.9012&1&0.9480\\
& Name&3&1&0.9745&0.9871&2&2&1&0.9953&0.9976\\
& Provider&2&1&1&1.00&2&2&1&1&1.00\\
& ReservationId&2&1&1&1.00&2&2&1&1&1.00\\
\hline\multirow{9}{*}{itinerary.westjet.com}
& ArrivalAirportIata&1&1&1&1.00&1&1&1&1&1.00\\
& ArrivalTime&1&1&1&1.00&1&1&1&1&1.00\\
& DepartureAirportIata&1&1&1&1.00&1&1&1&1&1.00\\
& DepartureDate&1&1&1&1.00&1&1&1&1&1.00\\
& DepartureTime&1&1&1&1.00&1&1&1&1&1.00\\
& FlightNumber&1&1&1&1.00&1&1&1&1&1.00\\
& Name&1&0.9931&1&0.9965&1&2&1&0.9942&0.9971\\
& Provider&1&1&1&1.00&1&1&1&1&1.00\\
& ReservationId&1&1&1&1.00&1&1&1&1&1.00\\
\hline\multirow{9}{*}{qatarairways.com.qa}
& ArrivalAirportIata&1&1&1&1.00&1&1&1&1&1.00\\
& ArrivalTime&1&1&1&1.00&1&1&1&1&1.00\\
& DepartureAirportIata&1&1&1&1.00&1&1&1&1&1.00\\
& DepartureDate&1&1&1&1.00&1&1&1&1&1.00\\
& DepartureTime&1&1&1&1.00&1&1&1&1&1.00\\
& FlightNumber&1&0.9982&1&0.9991&1&1&0.9982&1&0.9991\\
& Name&1&0.9988&1&0.9994&1&1&0.9988&1&0.9994\\
& Provider&1&1&1&1.00&1&1&1&1&1.00\\
& ReservationId&2&1&1&1.00&2&2&1&1&1.00\\
\hline
\end{tabular}
\caption{Results after adding new equivalence classes}
\end{table*}
%addition done to include equivalence classes
\begin{table*}[t]
\small
\label{table:m2hexpmt2-Add}
\begin{tabular}{|c|c|c|c|c|c|c|c|}
\hline
{Domain} & \multicolumn{2}{c}{Original} &\multicolumn{2}{|c|}{Added} & \multicolumn{2}{|c|}{Final} & {New Equi Classes}\\
\cline{2-7}&  Train & Test & Train & Test & Train & Test& \\
\hline
delta&102&927&8&8&110&935&1\\
philippines&74&90&5&4&79&94&4\\
qatar&55&581&10&20&65&601&9\\
westjet&50&427&5&73&55&500&0\\
\hline
\end{tabular}
\caption{Additions made to the dataset to account for out of cluster entities}
\end{table*}

\begin{table*}
\small
\label{table:m2hexpmt2}
\resizebox{17cm}{!}{
\begin{tabular}{|l|c|l|}
\hline
Domain : Field &  & Program\\

\hline\multirow{3}{*}{ifly.alaskaair.com:ArrivalAirportIata}
&HDEF&$TR:nth-child(1):nth-last-child(1) > [style*="width\:48\%"]:nth-child(3) > TABLE[cellpadding="0"][cellspacing="0"][border="0"][style*="width\:100\%"]:nth-child(1):nth-last-child(1) > TBODY:nth-child(1):nth-last-child(1) > :nth-child(1)$\\
& &$TR:nth-child(1):nth-last-child(1) > [style*="padding-bottom\:25px"] > TABLE[cellpadding="0"][cellspacing="0"][border="0"][style*="width\:100\%"]:nth-child(1):nth-last-child(1) > TBODY:nth-child(1):nth-last-child(1) > :nth-last-child(4)$\\
& HiSyn &$TR:nth-child(1)$ \\

\hline\multirow{4}{*}{ifly.alaskaair.com:DepartureTime}
&HDEF&$TR:nth-child(1):nth-last-child(1) > [style*="width\:48\%"]:nth-child(1) > TABLE[cellpadding="0"][cellspacing="0"][border="0"][style*="width\:100\%"]:nth-child(1):nth-last-child(1) > TBODY:nth-child(1):nth-last-child(1) > :nth-child(2)$\\
& &$TR:nth-child(1):nth-last-child(1) > [style*="padding-bottom\:25px"] > TABLE[cellpadding="0"][cellspacing="0"][border="0"][style*="width\:100\%"]:nth-child(1):nth-last-child(1) > TBODY:nth-child(1):nth-last-child(1) > :nth-last-child(3)$ \\ 
& HiSyn &$:nth-child(2)$ \\
\hline\multirow{2}{*}{ifly.alaskaair.com:ReservationID}
&HDEF&$TR:nth-child(1):nth-last-child(1) > [style*="padding-bottom\:20px"] > [align="center"] > TBODY:nth-child(1):nth-last-child(1) > :nth-child(1)$\\
&HiSyn&$TR:nth-child(1)$\\

\hline\multirow{2}{*}{delta.com:DepartureAirportIata}
&HDEF&$TABLE:nth-child(1) > TBODY:nth-child(1):nth-last-child(1) > TR > [style*="font-family\:Lucida Grande\, Lucida Sans\, Lucida Sans Unicode\, Trebuchet MS\, Verdana\, Tahoma\, sans-serif"]:nth-last-child(4) > SPAN[style*="color\:rgb(112, 112, 112)"]:nth-child(1):nth-last-child(1)$\\
&HiSyn&$TBODY > TR > :nth-child(3)$\\

\hline\multirow{2}{*}{delta.com:DepartureAirportIata}
&HDEF&$TABLE:nth-child(1) > TBODY:nth-child(1):nth-last-child(1) > TR > [style*="font-family\:Lucida Grande\, Lucida Sans\, Lucida Sans Unicode\, Trebuchet MS\, Verdana\, Tahoma\, sans-serif"]:nth-last-child(4) > SPAN[style*="color\:rgb(112, 112, 112)"]:nth-child(1):nth-last-child(1)$\\
&HiSyn&$TBODY > TR > :nth-child(3)$ \\

\hline\multirow{2}{*}{booking.airasia.com:DepartureTime} 
&HDEF &$ [style*="border-collapse\:collapse"][style*="font-family\:Roboto\, Arial\, sans-serif"] > TBODY:nth-child(1):nth-last-child(1) > :nth-last-child(1):nth-child(1) > [valign="middle"]:nth-child(3) > :nth-child(3)$\\
&HiSyn&$TD:nth-child(3) > :nth-child(3)$ \\

\hline\multirow{2}{*}{getthere.com:Provider} & HDEF&
$DIV:nth-last-child(13) > TABLE > TBODY:nth-child(1):nth-last-child(1) > :nth-child(1) > :nth-child(2)$\\&HiSyn&$:nth-child(2)$\\
\hline\multirow{2}{*}{getthere.com:ReservationID} & HDEF &
$:nth-last-child(17) > TABLE > TBODY:nth-child(1):nth-last-child(1) > :nth-child(2) > :nth-child(2)$\\&HiSyn&$:nth-child(2)$\\
\hline\multirow{2}{*}{t.delta.com:DepartureAirportIata}
&HDEF&$.mj-column-per-100 > TABLE[border="0"][cellpadding="0"][cellspacing="0"][role="presentation"]:nth-child(1):nth-last-child(1) > TBODY:nth-child(1):nth-last-child(1) > TR > :nth-child(2)$\\&HiSyn&$TBODY:nth-child(1):nth-last-child(1) > TR > :nth-child(2)$\\
\hline\multirow{2}{*}{t.delta.com:DepartureTime}
&HDEF&$.mj-column-per-100 > :nth-child(1):nth-last-child(1) > TBODY:nth-child(1):nth-last-child(1) > TR > :nth-child(2)$\\&HiSyn&$TBODY:nth-child(1):nth-last-child(1) > TR > :nth-child(2)$\\

\hline\multirow{2}{*}{philippineairlines.com:Name}
&HDEF &$.content > [cellpadding="2"] > TBODY:nth-child(1):nth-last-child(1) > [valign="top"] > :nth-last-child(4):nth-child(1)$
\\&HiSyn&$TR:nth-last-child(29)$\\

\hline\multirow{2}{*}{itinerary.westjet.com:DepartureAirportIata} 
&HDEF&$[style*="font-size\:13px"][width="100\%"] > TBODY:nth-child(1):nth-last-child(1) > :nth-last-child(3):nth-child(1) > .accent > [id*="airSegment-departure-city-"]$\\&HiSyn&$.accent > SPAN[id*="airSegment-departure-city-"][style*="text-transform\:uppercase"]:nth-child(1)$\\

\hline\multirow{2}{*}{aeromexico.com:ArrivalTime} &HDEF &
$[id*="itinerary-container"] > TABLE[cellspacing="0"][width="100\%"]:nth-child(1):nth-last-child(1) > TBODY:nth-child(1):nth-last-child(1) > [style*="vertical-align\:top"] > [id*="-arrival-time"]$\\&HiSyn&$TBODY:nth-child(1):nth-last-child(1) > [style*="vertical-align\:top"] > [id*="-arrival-time"]$\\

\hline\multirow{2}{*}{mytrips.amexgbt.com:FlightNumber} 
&HDEF&$TBODY > :nth-child(1):nth-last-child(1) > :nth-child(2) > DIV.right_section:nth-child(1):nth-last-child(1) > :nth-child(7):nth-last-child(12)$\\&HiSyn&$P:nth-child(7):nth-last-child(12)$ \\

\hline\multirow{2}{*}{mytrips.amexgbt.com:FlightNumber}&HDEF&
$TBODY > :nth-child(1):nth-last-child(1) > :nth-child(2) > DIV.right_section:nth-child(1):nth-last-child(1) > :nth-child(7):nth-last-child(12)$ \\&HiSyn& $P:nth-child(7):nth-last-child(12)$ \\

\hline\multirow{2}{*}{qatarairways.com.qa:DepartureDate} 
&HDEF&$[style*="margin-bottom\:10px"]:nth-child(2) >  TBODY:nth-child(1):nth-last-child(1) > TR:nth-child(1):nth-last-child(1) > :nth-child(4)$\\&HiSyn&$TABLE > TBODY:nth-child(1):nth-last-child(1) > TR:nth-child(1):nth-last-child(1) > :nth-child(4)$\\

\hline
\end{tabular}
}
\caption{HDEF vs ReSyn Programs}
\end{table*}
