# Supplementary material for: Landmarks and Regions: A Robust Approach to Data Extraction
Source: arXiv:2204.05021 source file (2022-04-11)
Supplement: Supplementary file 2 [file supplementary.tex]

\begin{table*}
\small
\label{table:m2hexpmt2}
\begin{tabular}{|l|}
\hline
ifly.alaskaair.com : ArrivalAirportIata \\
\\
$\ndsyn$: \\
$L_{ex}$: $TR:nth-child(1):nth-last-child(1) > [style*="width:48\%"]:nth-child(3) >  TABLE[cellpadding="0"]$ 
\\
$[cellspacing="0"][border=0][style*="width:100\%"]:nth-child(1):nth-last-child(1) >$
\\
$TBODY:nth-child(1):nth-last-child(1) > :nth-child(1)$\\
$Text Program$ : $Extract(str, RegexPair("\epsilon", "Alphanumeric"), RegexPair("Alphanumeric", "\epsilon"), -1)$\\
\smallskip\\
$\resyn$:\\
$Landmark$ : $Arrives$\\
$L_{rg}$: $\langle \mathsf{parenthops}: 0, \mathsf{siblinghops}$: $1$, $\mathsf{blueprint}$ : /TR/TD  $\rangle$\\
$L_{ex}$: $TR:nth-child(1)$ \\
$Text Program$ : $Extract(str, RegexPair("\epsilon", "Alphanumeric"), RegexPair("Alphanumeric", "\epsilon"),1)$ \\
\hline
getthere.com:Provider \\
\\
$\ndsyn$: \\
$L_{ex}$: $DIV:nth-last-child(13) > TABLE > TBODY:nth-child(1):nth-last-child(1) > :nth-child(1) > :nth-child(2)$ \\
$Text Program$ : $Extract(str, RegexPair(\epsilon, "Alphanumeric"), RegexPair(\epsilon, "WhiteSpaceNumber"), 1)$\\
\\ 
$\resyn$:\\
$Landmark$ : $Flight/Equip$\\
$L_{rg}:\langle \mathsf{parenthops}: 0, \mathsf{siblinghops}: 1, \mathsf{blueprint}:/TD  \rangle$\\
$L_{ex}:nth-child(2)$ \\
$Text Program$ : $Extract(str, RegexPair(\epsilon, "Alphanumeric"), RegexPair($\epsilon$, "WhiteSpaceNumber"), 1)$\\

\smallskip \\
\hline
booking.airasia.com:DepartureDate \\
\\
$\ndsyn$:\\
$L_{ex}$ : $[style*="border-collapse\:collapse"][style*="font-family\:Roboto\, Arial\, sans-serif"] >$\\$ TBODY:nth-child(1):nth-last-child(1) > :nth-last-child(1):nth-child(1) > [valign="middle"]:nth-child(3) > :nth-child(3)$
\\ 
$:nth-child(1):nth-last-child(1) > :nth-last-child(1):nth-child(1) > [valign="middle"]:nth-child(3)$ \\
$ > :nth-child(3)$ \\
$Text Program$:$Extract(str,RegexPair("","WhiteSpace"),RegexPair("\epsilon","LineSeperator"),-1)$\\
\\
$\resyn$: 
\\
$Landmark$ :$Depart$\\
$L_{rg}:\langle \mathsf{parenthops}: 1, \mathsf{siblinghops}: 2, \mathsf{blueprint}:/TD/SPAN/TD/SPAN  \rangle$\\
$L_{ex}$:$TD:nth-child(3) > :nth-child(3)$ \\
$Text Program$:$Extract(str,RegexPair("","WhiteSpace"),RegexPair("\epsilon","LineSeperator"),-1)$\\
\hline
\end{tabular}
\end{table*}

\begin{table*}
\small
\label{table:m2hlandmarks}
\begin{tabular}{|l|l|l|}
\hline
{Domain} & User provided landmarks & Learnt landmarks \\
\hline

ifly.alaskaair & 

Departs, Arrives, Term/Gate,  & Departs, Arrives, \textbf{Confirmation code: >> Term/Gate,}  \\

   & Travellers, Confirmation code &  Travellers, \textbf{Travelers: >> Confirmation code}  \\
\hline
delta & To, Arrival Time, Flight, Departs, & To, Arrival Time, Flight, Departs,  \\

& Departure Time, Flight, Flight Number:,  & Departure Time, Flight, Flight Number:, \\

& Name, Who's coming along, Carrier, & Name, Who's coming along, Carrier,  \\

& Confirmation Number:, Record Locator:  & Confirmation Number:, Record Locator: \\

\hline
booking.airasia & Arrive, Depart, Guests, Booking number & Arrive, Depart, Guests, Booking number \\

\hline
getthere.com & Arrive: , Depart:, Fligt/Equip, Name,  & Arrive: , Depart:, Fligt/Equip, \textbf{Meal >> Name,}  \\

& Airline Record Locator & Airline Record Locator \\ 

\hline
qatarairways & Destination:, Arriving:, Origin:, Departing:,  & Destination:, Arriving:, Origin:, Departing:, Class,  \\

& Class, Passenger name, Booking reference (PNR) & Passenger name, Booking reference (PNR) \\
\hline
\end{tabular}

\end{table*}

\begin{table*}
\small
\begin{tabular}{|c|l|c|c|c||c|c|c|}
\hline
 & & \multicolumn{3}{|c|}{ \ndsyn} &  \multicolumn{3}{|c|}{\resyn} \\
 {Domain} & Fields & $Prec$ & $Recall$& $F1$ & $Prec$ & $Recall$& $F1$ \\
\hline
\hline\multirow{8}{*}{iflyalaskaair}

& AIata & 1.00 & 0.68 & 0.81 & 1.00 & 1.00 & 1.00 \\
& ATime & 0.94 & 0.63 & 0.76 & 1.00 & 1.00 & 1.00 \\
& DIata & 1.00 & 0.58 & 0.73 & 1.00 & 1.00 & 1.00 \\
& DDate & 1.00 & 1.00 & 1.00 & 1.00 & 1.00 & 1.00 \\
& DTime & 1.00 & 0.58 & 0.73 & 1.00 & 1.00 & 1.00 \\
& FNum  & 1.00 & 1.00 & 1.00 & 1.00 & 1.00 & 1.00 \\
& Name  & 1.00 & 1.00 & 1.00 & 1.00 & 1.00 & 1.00 \\
& RId   & 1.00 & 1.00 & 1.00 & 1.00 & 1.00 & 1.00 \\

\hline\multirow{9}{*}{airasia}

& AIata & 0.50 & 1.00 & 0.67 & 1.00 & 1.00 & 1.00 \\
& ATime & 0.00 & 0.00 & 0.00 & 1.00 & 1.00 & 1.00 \\
& DIata & 0.50 & 1.00 & 0.67 & 1.00 & 1.00 & 1.00 \\
& DDate & 0.50 & 1.00 & 0.67 & 1.00 & 1.00 & 1.00 \\
& DTime & 0.00 & 0.00 & 0.00 & 1.00 & 1.00 & 1.00 \\
& FNum  & 1.00 & 1.00 & 1.00 & 1.00 & 1.00 & 1.00 \\
& Name  & 1.00 & 1.00 & 1.00 & 1.00 & 1.00 & 1.00 \\
& Pvdr  & 1.00 & 1.00 & 1.00 & 1.00 & 1.00 & 1.00 \\
& RId   & 1.00 & 1.00 & 1.00 & 1.00 & 1.00 & 1.00 \\

\hline\multirow{9}{*}{getthere}

& AIata & 0.81 & 0.70 & 0.75 & 1.00 & 1.00 & 1.00 \\
& ATime & 0.96 & 0.91 & 0.94 & 1.00 & 1.00 & 1.00 \\
& DIata & 0.96 & 0.92 & 0.94 & 1.00 & 1.00 & 1.00 \\
& DDate & 0.99 & 0.96 & 0.98 & 1.00 & 1.00 & 1.00 \\
& DTime & 0.87 & 0.67 & 0.76 & 1.00 & 1.00 & 1.00 \\
& FNum & 1.00 & 0.96 & 0.98 & 1.00 & 1.00 & 1.00 \\
& Name & 1.00 & 1.00 & 1.00 & 1.00 & 1.00 & 1.00 \\
& Pvdr & 1.00 & 0.96 & 0.98 & 1.00 & 1.00 & 1.00 \\
& RId & 1.00 & 0.87 & 0.93 & 1.00 & 1.00 & 1.00 \\

\hline\multirow{9}{*}{delta}
& AIata & 1.00 & 1.00 & 1.00 & 1.00 & 1.00 & 1.00 \\
& ATime & 1.00 & 1.00 & 1.00 & 1.00 & 1.00 & 1.00 \\
& DIata & 1.00 & 1.00 & 1.00 & 1.00 & 1.00 & 1.00 \\
& DDate & 0.91 & 0.97 & 0.94 & 1.00 & 1.00 & 1.00 \\
& DTime & 1.00 & 1.00 & 1.00 & 1.00 & 1.00 & 1.00 \\
& FNum & 1.00 & 1.00 & 1.00 & 1.00 & 1.00 & 1.00 \\
& Name & 0.92 & 0.80 & 0.85 & 0.93 & 1.00 & 0.97 \\
& Pvdr & 1.00 & 1.00 & 1.00 & 1.00 & 1.00 & 1.00 \\
& RId & 1.00 & 1.00 & 1.00 & 1.00 & 1.00 & 1.00 \\

\hline\multirow{9}{*}{aeromexico}
 & AIata & 1.00 & 1.00 & 1.00 & 1.00 & 1.00 & 1.00 \\
 & ATime & 1.00 & 1.00 & 1.00 & 1.00 & 1.00 & 1.00 \\
 & DIata & 1.00 & 1.00 & 1.00 & 1.00 & 1.00 & 1.00 \\
 & DDate & 1.00 & 1.00 & 1.00 & 1.00 & 1.00 & 1.00 \\
 & DTime & 1.00 & 1.00 & 1.00 & 1.00 & 1.00 & 1.00 \\
 & FNum & 1.00 & 1.00 & 1.00 & 1.00 & 1.00 & 1.00 \\
 & Name & 1.00 & 1.00 & 1.00 & 1.00 & 1.00 & 1.00 \\
 & Pvdr & 1.00 & 1.00 & 1.00 & 1.00 & 1.00 & 1.00 \\
 & RId & 1.00 & 1.00 & 1.00 & 1.00 & 1.00 & 1.00 \\

\hline\multirow{9}{*}{mytrips.amexgbt}
 & AIata & 1.00 & 1.00 & 1.00 & 1.00 & 1.00 & 1.00 \\
 & ATime & 1.00 & 1.00 & 1.00 & 1.00 & 1.00 & 1.00 \\
 & DIata & 1.00 & 1.00 & 1.00 & 1.00 & 1.00 & 1.00 \\
 & DDate & 1.00 & 1.00 & 1.00 & 1.00 & 1.00 & 1.00 \\
 & DTime & 1.00 & 1.00 & 1.00 & 1.00 & 1.00 & 1.00 \\
 & FNum & 1.00 & 1.00 & 1.00 & 1.00 & 1.00 & 1.00 \\
 & Name & 1.00 & 1.00 & 1.00 & 1.00 & 1.00 & 1.00 \\
 & Pvdr & 1.00 & 1.00 & 1.00 & 1.00 & 1.00 & 1.00 \\
 & RId & 1.00 & 1.00 & 1.00 & 1.00 & 1.00 & 1.00 \\

\hline 
\end{tabular}
\caption{M2H Contemporary}
\label{tab:m2hexpmt1}
\end{table*}

\begin{table*}
\small
\begin{tabular}{|c|l|c|c|c||c|c|c|}
\hline
 & & \multicolumn{3}{|c||}{ \ndsyn} &  \multicolumn{3}{|c|}{\resyn} \\
 {Domain} & Fields & $Prec$ & $Recall$& $F1$ & $Prec$ & $Recall$ & $F1$ \\
\hline
\hline\multirow{8}{*}{iflyalaskaair}

& AIata & 1.00 & 0.47 & 0.64  & 1.00 & 1.00 & 1.00 \\
& ATime & 1.00 & 0.47 & 0.64  & 1.00 & 1.00 & 1.00 \\
& DIata & 1.00 & 0.38 & 0.55  & 1.00 & 1.00 & 1.00 \\
& DDate & 1.00 & 1.00 & 1.00  & 1.00 & 1.00 & 1.00 \\
& DTime & 1.00 & 0.38 & 0.55  & 1.00 & 1.00 & 1.00 \\
& FNum  & 1.00 & 1.00 & 1.00  & 1.00 & 1.00 & 1.00 \\
& Name  & 1.00 & 0.98 & 0.99  & 1.00 & 0.98 & 0.99 \\
& RId   & 1.00 & 1.00 & 1.00  & 1.00 & 1.00 & 1.00 \\

\hline\multirow{9}{*}{airasia}

& AIata & 0.50 & 1.00 & 0.67 & 1.00 & 1.00 & 1.00 \\
& ATime & 0.00 & 0.00 & 0.00 & 1.00 & 1.00 & 1.00 \\
& DIata & 0.50 & 1.00 & 0.67 & 1.00 & 1.00 & 1.00 \\
& DDate & 0.50 & 1.00 & 0.67 & 1.00 & 1.00 & 1.00 \\
& DTime & 0.00 & 0.00 & 0.00 & 1.00 & 1.00 & 1.00 \\
& FNum  & 1.00 & 0.92 & 0.96 & 1.00 & 0.92 & 0.96 \\
& Name  & 1.00 & 1.00 & 1.00 & 1.00 & 1.00 & 1.00 \\
& Pvdr  & 1.00 & 0.92 & 0.96 & 1.00 & 0.92 & 0.96 \\
& RId   & 1.00 & 1.00 & 1.00 & 1.00 & 1.00 & 1.00 \\

\hline\multirow{9}{*}{getthere}

& AIata & 0.76 & 0.71 & 0.74 & 1.00 & 1.00 & 1.00 \\
& ATime & 0.95 & 0.88 & 0.91 & 1.00 & 1.00 & 1.00 \\
& DIata & 0.99 & 0.90 & 0.95 & 1.00 & 1.00 & 1.00 \\
& DDate & 0.99 & 0.91 & 0.95 & 1.00 & 1.00 & 1.00 \\
& DTime & 0.85 & 0.73 & 0.78 & 1.00 & 1.00 & 1.00 \\
& FNum & 0.99 & 0.96 & 0.98 & 1.00 & 1.00 & 1.00 \\
& Name & 0.83 & 0.96 & 0.89 & 1.00 & 1.00 & 1.00 \\
& Pvdr & 1.00 & 0.95 & 0.97 & 1.00 & 1.00 & 1.00 \\
& RId & 1.00 & 0.88 & 0.94 & 1.00 & 1.00 & 1.00 \\

\hline\multirow{9}{*}{delta}
& AIata & 1.00 & 1.00 & 1.00 & 1.00 & 1.00 & 1.00 \\
& ATime & 1.00 & 1.00 & 1.00 & 1.00 & 1.00 & 1.00 \\
& DIata & 1.00 & 1.00 & 1.00 & 1.00 & 1.00 & 1.00 \\
& DDate & 0.94 & 0.97 & 0.95 & 1.00 & 1.00 & 1.00 \\
& DTime & 1.00 & 1.00 & 1.00 & 1.00 & 1.00 & 1.00 \\
& FNum & 1.00 & 1.00 & 1.00 & 1.00 & 1.00 & 1.00 \\
& Name & 0.94 & 0.88 & 0.91 & 0.95 & 1.00 & 0.97 \\
& Pvdr & 1.00 & 1.00 & 1.00 & 1.00 & 1.00 & 1.00 \\
& RId & 1.00 & 1.00 & 1.00 & 1.00 & 1.00 & 1.00 \\

\hline\multirow{9}{*}{aeromexico}
 & AIata & 1.00 & 1.00 & 1.00 & 1.00 & 1.00 & 1.00 \\
 & ATime & 1.00 & 1.00 & 1.00 & 1.00 & 1.00 & 1.00 \\
 & DIata & 1.00 & 1.00 & 1.00 & 1.00 & 1.00 & 1.00 \\
 & DDate & 1.00 & 1.00 & 1.00 & 1.00 & 1.00 & 1.00 \\
 & DTime & 1.00 & 1.00 & 1.00 & 1.00 & 1.00 & 1.00 \\
 & FNum & 1.00 & 1.00 & 1.00 & 1.00 & 1.00 & 1.00 \\
 & Name & 1.00 & 1.00 & 1.00 & 1.00 & 1.00 & 1.00 \\
 & Pvdr & 1.00 & 1.00 & 1.00 & 1.00 & 1.00 & 1.00 \\
 & RId & 1.00 & 1.00 & 1.00 & 1.00 & 1.00 & 1.00 \\

\hline\multirow{9}{*}{mytrips.amexgbt}
 & AIata & 1.00 & 1.00 & 1.00 & 1.00 & 1.00 & 1.00 \\
 & ATime & 1.00 & 1.00 & 1.00 & 1.00 & 1.00 & 1.00 \\
 & DIata & 1.00 & 1.00 & 1.00 & 1.00 & 1.00 & 1.00 \\
 & DDate & 1.00 & 1.00 & 1.00 & 1.00 & 1.00 & 1.00 \\
 & DTime & 1.00 & 1.00 & 1.00 & 1.00 & 1.00 & 1.00 \\
 & FNum & 1.00 & 1.00 & 1.00 & 1.00 & 1.00 & 1.00 \\
 & Name & 1.00 & 1.00 & 1.00 & 1.00 & 1.00 & 1.00 \\
 & Pvdr & 1.00 & 1.00 & 1.00 & 1.00 & 1.00 & 1.00 \\
 & RId & 1.00 & 1.00 & 1.00 & 1.00 & 1.00 & 1.00 \\

\hline 
\end{tabular}
\caption{M2H Longitudinal}
\label{tab:m2hexpmt1}
\end{table*}

\begin{table*}
\small
\begin{tabular}{|c|l|c|c|c|c||c|c|c|c|}
\hline
 & & \multicolumn{4}{|c||}{ \afr} &  \multicolumn{4}{|c|}{\resyn} \\
 {Domain} & Fields & $Prec$ & $Recall$& $F1$ & $Acc$ & $Prec$ & $Recall$& $F1$ & $Acc$ \\
\hline
 \hline\multirow{9}{*}{aeromexico.com} 
 & AIata & 0.62 & 0.51 & 0.80 & 0.28 & 0.65 & 0.98 & 0.49 & 0.36 \\
 & ATime & 0.69 & 0.81 & 0.61 & 0.43 & 0.99 & 1.00 & 0.99 & 0.93 \\
 & DIata & 0.36 & 0.37 & 0.35 & 0.31 & 0.66 & 1.00 & 0.49 & 0.37 \\
 & DDate & 0.71 & 0.70 & 0.72 & 0.37 & 0.89 & 0.90 & 0.88 & 0.58 \\
 & DTime & 0.65 & 0.82 & 0.54 & 0.31 & 0.97 & 1.00 & 0.94 & 0.76\\
 & FNum & 0.66 & 0.55 & 0.82 & 0.52 & 0.83 & 0.71 & 1.00 & 0.75 \\
 & Name & 0.96 & 0.95 & 0.98 & 0.74 & 0.98 & 0.97 & 1.00 & 0.80\\
 & Pvdr & 0.69 & 0.62 & 0.79 & 0.43 & 0.78 & 0.67 & 0.94 & 0.72 \\
 & RId & 1.00 & 1.00 & 1.00 & 1.00 & 1.00 & 1.00 & 1.00 & 1.00 \\
 
 \hline\multirow{9}{*}{getthere.com}   
 & AIata & 0.94 & 0.99 & 0.89 & 0.81 & 1.00 & 1.00 & 1.00 & 0.99 \\
 & ATime & 0.87 & 0.98 & 0.79 & 0.50 & 1.00 & 1.00 & 1.00 & 1.00 \\
 & DIata & 0.93 & 1.00 & 0.87 & 0.72 & 1.00 & 0.99 & 1.00 & 0.98 \\
 & DDate & 0.96 & 0.97 & 0.95 & 0.85 & 0.99 & 0.98 & 1.00 & 0.94 \\
 & DTime & 0.88 & 1.00 & 0.79 & 0.55 & 1.00 & 1.00 & 1.00 & 1.00 \\
 & FNum & 0.94 & 0.94 & 0.94 & 0.82 & 1.00 & 1.00 & 1.00 & 0.99 \\
 & Name & 0.99 & 0.98 & 1.00 & 0.94 & 0.99 & 0.98 & 1.00 & 0.92 \\
 & Pvdr & 0.75 & 0.62 & 0.94 & 0.31 & 1.00 & 1.00 & 1.00 & 0.99 \\
 & RId & 0.89 & 0.93 & 0.85 & 0.81 &  0.95 & 0.99 & 0.91 & 0.90 \\
 
 \hline\multirow{9}{*}{itinerary.westjet} 
 & AIata & 0.94 & 0.96 & 0.93 & 0.81 &   0.99 & 0.99 & 0.99 & 0.95 \\
 & ATime & 0.90 & 0.86 & 0.95 & 0.68 &   0.88 & 0.92 & 0.85 & 0.72 \\
 & DIata & 0.93 & 0.94 & 0.93 & 0.78 &   0.98 & 0.98 & 0.99 & 0.93 \\
 & DDate & 0.93 & 0.90 & 0.95 & 0.72 &   1.00 & 1.00 & 1.00 & 0.99 \\
 & DTime & 0.94 & 0.92 & 0.97 & 0.82 &   0.95 & 0.95 & 0.95 & 0.83 \\
 & FNum & 0.96 & 0.97 & 0.95 & 0.90 &   1.00 & 1.00 & 1.00 & 1.00 \\
 & Name & 0.60 & 0.44 & 0.92 & 0.00 &   0.61 & 0.47 & 0.88 & 0.01 \\
 & Pvdr & 0.95 & 0.96 & 0.94 & 0.89 &   1.00 & 1.00 & 1.00 & 0.99 \\
 & RId & 1.00 & 1.00 & 1.00 & 1.00 &   1.00 & 1.00 & 1.00 & 1.00 \\
 
 \hline\multirow{9}{*}{mytrips.amexgbt}   
 & AIata & 0.85 & 0.74 & 0.98 & 0.89 & 0.98 & 0.99 & 0.97 & 0.94 \\
 & ATime & 0.97 & 0.95 & 0.99 & 0.95 & 1.00 & 1.00 & 1.00 & 1.00 \\
 & DIata & 0.96 & 0.96 & 0.95 & 0.91 & 0.99 & 0.99 & 0.99 & 0.97 \\
 & DDate & 0.93 & 0.87 & 0.99 & 0.72 & 1.00 & 1.00 & 1.00 & 0.99 \\
 & DTime & 0.99 & 0.99 & 0.99 & 0.95 & 1.00 & 1.00 & 1.00 & 1.00 \\
 & FNum & 0.98 & 0.98 & 0.99 & 0.95 & 1.00 & 1.00 & 1.00 & 1.00 \\
 & Name & 0.98 & 0.98 & 0.98 & 0.97 & 1.00 & 1.00 & 1.00 & 1.00 \\
 & Pvdr & 0.91 & 0.85 & 0.99 & 0.89 & 0.99 & 0.98 & 0.99 & 0.97 \\
 & RId & 0.61 & 0.47 & 0.89 & 0.65 & 0.96 & 0.98 & 0.95 & 0.92 \\

\hline
\end{tabular}
\caption{Scores for Images M2H Dataset}
\label{tab:imagesm2h}
\end{table*}

\begin{table*}
\small
\begin{tabular}{|c|l|c|c|c|c||c|c|c|c|}
\hline
 & & \multicolumn{4}{|c||}{ \afr} &  \multicolumn{4}{|c|}{\resyn} \\
 {Domain} & Fields & $Prec$ & $Recall$& $F1$ & $Acc$ & $Prec$ & $Recall$& $F1$ & $Acc$ \\
\hline
\hline\multirow{9}{*}{AccountsInvoice}
  & Amount & 0.99 & 0.99 & 0.99 & 0.99 & 1.00 & 1.00 & 1.00 & 1.00 \\
  & Chassis & 0.82 & 0.82 & 0.81 & 0.66 & 0.94 & 0.99 & 0.91 & 0.48 \\
  & CustAddr & 0.98 & 0.99 & 0.98 & 0.78 & 0.96 & 0.96 & 0.97 & 0.83 \\
  & Date & 0.93 & 0.95 & 0.91 & 0.92 & 0.98 & 0.99 & 0.97 & 0.97 \\
  & Dnum & 0.96 & 0.98 & 0.94 & 0.96 & 0.97 & 0.99 & 0.96 & 0.95 \\
  & Engine & 0.82 & 0.76 & 0.88 & 0.90 & 1.00 & 1.00 & 1.00 & 1.00 \\
  & InvoiceAddress & 0.90 & 0.97 & 0.83 & 0.50 & 0.95 & 0.98 & 0.91 & 0.32 \\
  & Model & 0.75 & 0.90 & 0.64 & 0.63 & 1.00 & 1.00 & 1.00 & 0.99 \\

\hline\multirow{8}{*}{CashInvoice}
  & Amount & 1.00 & 1.00 & 1.00 & 1.00 & 1.00 & 1.00 & 1.00 & 1.00 \\
  & Chassis & 0.99 & 0.99 & 0.98 & 0.95 & 0.99 & 1.00 & 0.98 & 0.97 \\
  & CustAddr & 0.99 & 0.99 & 0.99 & 0.85 & 0.97 & 0.94 & 0.99 & 0.80 \\
  & Date & 0.99 & 1.00 & 0.98 & 0.98 & 0.99 & 1.00 & 0.98 & 0.98 \\
  & Dnum & 0.96 & 0.98 & 0.95 & 0.98 & 0.96 & 0.97 & 0.95 & 0.94 \\
  & Engine & 0.93 & 0.93 & 0.93 & 0.93 & 0.95 & 0.93 & 0.96 & 0.93 \\
  & InvoiceAddress & 0.99 & 0.99 & 0.99 & 0.85 & 0.99 & 1.00 & 0.98 & 0.85 \\
  & Model & 0.99 & 1.00 & 0.99 & 0.95 & 1.00 & 1.00 & 1.00 & 1.00 \\

\hline\multirow{5}{*}{CreditNote}
  & Amount & 1.00 & 1.00 & 1.00 & 1.00 & 1.00 & 1.00 & 1.00 & 1.00 \\
  & CreditNoteAddress & 0.99 & 0.98 & 0.99 & 0.93 & 1.00 & 0.99 & 1.00 & 0.97 \\
  & CreditNoteNo & 0.94 & 1.00 & 0.88 & 0.93 & 0.93 & 0.98 & 0.88 & 0.85 \\
  & CustRefNo & 1.00 & 1.00 & 1.00 & 1.00 & 1.00 & 1.00 & 1.00 & 1.00 \\
  & Date & 1.00 & 1.00 & 1.00 & 1.00 & 1.00 & 1.00 & 1.00 & 1.00 \\
  & RefNo & 1.00 & 1.00 & 1.00 & 1.00 & 1.00 & 1.00 & 1.00 & 1.00 \\

\hline\multirow{6}{*}{SalesInvoice}
  & Amount & 1.00 & 1.00 & 1.00 & 1.00 & 1.00 & 1.00 & 1.00 & 1.00 \\
  & CustomerReferenceNo & 1.00 & 1.00 & 1.00 & 1.00 & 1.00 & 1.00 & 1.00 & 1.00 \\
  & Date & 1.00 & 1.00 & 1.00 & 0.99 & 1.00 & 1.00 & 1.00 & 1.00 \\
  & InvoiceAddress & 0.94 & 0.98 & 0.90 & 0.67 & 0.99 & 1.00 & 0.99 & 0.95 \\
  & RefNo & 0.99 & 0.99 & 0.99 & 0.99 & 0.99 & 1.00 & 0.99 & 0.99 \\
  & SalesInvoiceNo & 0.99 & 1.00 & 0.99 & 1.00 & 0.99 & 1.00 & 0.98 & 0.99 \\

\hline\multirow{6}{*}{SelfBilledCreditNote}
  & Amount & 1.00 & 1.00 & 1.00 & 1.00 & 1.00 & 1.00 & 1.00 & 1.00 \\
  & CustomerAddress & 1.00 & 1.00 & 1.00 & 0.99 & 0.99 & 0.99 & 1.00 & 0.97 \\
  & CustomerReferenceNo & 0.99 & 0.99 & 0.99 & 0.99 & 0.99 & 1.00 & 0.97 & 0.97 \\
  & Date & 1.00 & 1.00 & 1.00 & 1.00 & 1.00 & 1.00 & 1.00 & 1.00 \\
  & DocumentNumber & 1.00 & 1.00 & 1.00 & 1.00 & 1.00 & 1.00 & 1.00 & 1.00 \\
  & VatRegNo & 1.00 & 1.00 & 1.00 & 1.00 & 1.00 & 1.00 & 1.00 & 1.00 \\

\hline
\end{tabular}
\caption{Scores for Finance dataset}
\label{tab:imagesdaimler}
\end{table*}

\begin{table*}
\small
\begin{tabular}{|l|}
\hline
Sale Invoice : Date \\
Landmark: "Date:" \\
Region program: Extend("Date", Relative(Right, EOL, false) \\
Text program: Extract a substring between ":" and EOL \\
\hline 
Accounts Invoice: Chassis Number \\
Landmark: "Chassis Number" \\
Region program: Extend(Extend(input, Absolute(down, 1)), Relative(Right, DATE, false)) \\
Text Program: Take all the strings in this path \\
\hline
Accounts Invoice : InvoiceAddress \\
Region program: ExtendLineItems("Invoice Name \& Address", Relative(down, "Model SKU")) \\
Text Program: Take all the strings in this path \\
\hline
\end{tabular}
\caption{Synthesized extraction programs \spsays{Improve presentation}}
\label{tab:imageprograms}
\end{table*}
